# Supplementary material for: Deep Forward and Inverse Perceptual Models for Tracking and Prediction
Source: arXiv:1710.11311 source file (2018-05-20)
Supplement: Supplementary file 1 [file appendix.tex]

\section{Appendix}
\subsection{GAN details}

We use a variant of the DC-GAN architecture from \cite{dcgan} for the current implementation, Joint-Conditioned GAN. The generator consists of 6 transposed convolution layer to generate a an image of size 256×256×3 from a latent vector of dimension 17. We use a 10 dimensional noise vector concatenated with a 7 dimensional joint angle acting as the conditioning signal. The discriminator is similar to [RMC15]. Both generator and discriminator are trained with a batch size of 32. Batch normalization is used to stabilize the training and for better quality of generated images. The images are mean-centered and centered cropped before training. The joint angles are also mean centered and normalized before using it as a conditioning signal. The mean and variance are cached at train time and the joint angle are normalized with these cached values at test time. We augment the GAN objective with L2 loss to stabilize the training: \( L_{total} = L_{GAN} + \lambda \L_{2}\)
The L2 loss is calculated with respect to the ground truth image for the corresponding joint angle.
The network is first trained with a high value of \(\lambda\) without adversarial objective for the first 5kiterations. This stabilizes the generated results. The discriminator is updated for the first 5k iterations but the generator is only updated with the L2 loss. After \(\lambda\) iterations λ is annealed as
follows:
λo
λ =
 (2)
1 + γ ∗ epoch
where γ is set to a low value such as 0.001
